# Supplementary material for: Single-atom transistor as a precise magnetic field sensor
Source: arXiv:1707.06018 source file (2018-01-04)
Supplement: Supplementary file 1 [file supplementary.pdf]

# Supplementary Material to “Single atom transistor as a precise magnetic field sensor


Krzysztof Jachymski[1], Tomasz Wasak[2], Zbigniew Idziaszek[2],
Paul S. Julienne[3], Antonio Negretti[4], and Tommaso Calarco[5]

[1] Institute for Theoretical Physics III & Center for Integrated Quantum Science and Technologies (IQST), University of Stuttgart, Pfaffenwaldring 57, 70550 Stuttgart, Germany
[2] Faculty of Physics, University of Warsaw, Pasteura 5, 02-093 Warsaw, Poland
[3] Joint Quantum Institute, University of Maryland and National Institute of Standards and Technolog, College Park, Maryland 20742, USA
[4] Zentrum für Optische Quantentechnologien and The Hamburg Centre for Ultrafast Imaging, Universität Hamburg, Luruper Chaussee 149, 22761 Hamburg, Germany
[5] Institute for Complex Quantum Systems & Center for Integrated Quantum Science and Technologies (IQST), Universität Ulm, 89069 Ulm, Germany



(Dated: October 27, 2017)



In this Supplementary Material we discuss the scattering problem in the presence of trapping potentials and the validity of Hamiltonian (1) from the main part of our work. Then we consider the effect of long-range dipolar interactions and higher partial waves. In the last part we investigate the optimality of our measurement scheme and show that the precision cannot be further improved by changing to a different scheme optionally preceded by any operation done on the state after the collision.


## I. ANHARMONIC TRAPS AND COUPLING TO THE CENTER OF MASS

We start with the general Hamiltonian describing the two particles in their respective trapping potentials

$$H=-\frac{\hbar^2}{2m_A}\Delta_A-\frac{\hbar^2}{2m_I}\Delta_I+V_A(\mathbf{r}_A)+V_I(\mathbf{r}_I)+U(\mathbf{r}_A-\mathbf{r}_I). \tag{1}$$

Here $A$ denotes the incoming atom, $I$ the impurity atom, and the interaction $U$ is described by the $s$-wave pseudopotential $U(r)=g\delta(r)\frac{\partial}{\partial r}r$ with $g=2\pi\hbar^2 a(B)/\mu$ with the reduced mass $\mu$ and free space $s$-wave scattering length $a(B)$ (effects of higher partial waves are discussed in the next section). The trapping lasers are weak and off-resonant so we omit small corrections they impose on the interaction (see e.g. [1]). It can be important to use the energy-dependent scattering length calculated at the actual collision energy [2] instead of the zero-energy limit.

The incoming atom is trapped by an optical lattice in two spatial dimensions, forming a quasi-one-dimensional waveguide $V_A(\mathbf{r_A})=\frac{1}{2}m_A\omega_A^2\rho_A^2$. Higher order corrections from the actual shape of the lattice can be accounted for in the numerical calculation [3, 4]. We assume that at large interparticle spacing the atom occupies the ground state of the transverse trap $\psi_0(\boldsymbol{\rho}_A)$, but finite temperature effects and other state preparation imperfections can also be accurately modelled numerically. In the main part of the manuscript we assume that the impurity atom is completely pinned in space and its dynamics can be neglected ($r_I=0$) so that the Hamiltonian reduces to

$$H=-\frac{\hbar^2}{2m_A}\Delta+V_A(\mathbf{r})+U(\mathbf{r}) \tag{2}$$

This reduces the problem to the well-known form first solved by Olshanii [5]. At large distances the wave function can be written as $\psi_0(\boldsymbol{\rho})\left(e^{ipz}+f(p)e^{ip|z|}\right)$ with the one-dimensional even scattering amplitude $f(p)$ which is linked to the phase shift by $f(p)=-\frac{1}{1+i\cot\delta(p)}$ and can be obtained analytically for harmonic potential.

It is important to relax the simplifying assumption of pinned impurity and check what one should expect in the general case. Typically, the impurity trapping potential can also be taken as a harmonic one $V_I(\mathbf{r}_I)=\frac{1}{2}m_I\omega_I^2r_I^2$ with higher order corrections that can be included in numerics. We also expect $\omega_I\gg\omega_A$. The center of mass and relative motion variables cannot be separated and the problem becomes in principle six-dimensional. However, at large interparticle distance the total wave function takes the separable form

$$\psi(\mathbf{r}_A,\mathbf{r}_I)\overset{|\mathbf{r}_A-\mathbf{r}_I|\to\infty}{\longrightarrow}\left(\psi_0(\boldsymbol{\rho}_A)\left(e^{ipz_A}+f(p)e^{ip|z_A|}\right)\right)\phi_0(\mathbf{r}_I). \tag{3}$$

This problem can be formally solved e.g. in terms of Green's function [6, 7]. The wave function is then given by

$$\psi(\mathbf{r}_A,\mathbf{r}_I)=\psi_f(\mathbf{r}_A,\mathbf{r}_I)+g\int d\mathbf{r}'G_E(\mathbf{r}_A,\mathbf{r}_I,\mathbf{r}',\mathbf{r}')\psi_{\rm reg}(\mathbf{r}'). \tag{4}$$

Here $G_E(\mathbf{r}_A,\mathbf{r}_I,\mathbf{r}',\mathbf{r}')$ is the Green's function of the noninteracting part of the full Hamiltonian (1) denoted as $H_0$

$$G_E=\frac{1}{E+i0^+-H_0}, \tag{5}$$

$\psi_f(\mathbf{r}_A,\mathbf{r}_I)=e^{ip_Az_A}\psi_0(\boldsymbol{\rho}_A)\phi_0(\mathbf{r}_I)$ denotes the solution of the noninteracting Hamiltonian, and the regularized wave function $\psi_{\rm reg}$ results from the interaction term in the Hamiltonian [6].

Numerical solution of this set of equations allows to

find the scattering amplitude $f(p)$ which is given by

$$f(p) = -\frac{m_A}{\mu} a(B) \int d^3\zeta \cos(p\zeta_z) \psi_0(\zeta_\rho) \phi_0(\boldsymbol{\zeta}) \psi_{\rm reg}(\boldsymbol{\zeta}). \tag{6}$$

We notice that assuming the pinned impurity case, $\phi_0(\boldsymbol{\zeta})$ is replaced by a Dirac delta and the integral is reduced to the product of the regularized part of the wave function and the transverse trap state calculated at the origin, exactly as in the solution of the separable problem [5].

The knowledge of $f(p)$ allows for computing the transmission which is the key quantity in our sensing protocol. Let us now discuss what features can be expected from the full numerical solution. First, one finds a shift of the scattering amplitude resulting from the trapping potentials, which is also the case for the pure harmonic waveguide [5] or optical lattice [7]. This shift should be included in the description to ensure high accuracy, but does not fundamentally affect the properties of the system. The next effect is the emergence of multiple resonances in the one-dimensional scattering length [6]. To explain this, we note that the full Hamiltonian couples the center of mass and relative motion. Let us consider a simple illustrative picture and consider the case where the particles are close to each other and we can neglect $\omega_A$ compared to $\omega_B$. We then have

$$H \approx -\frac{\hbar^2 \Delta_R}{2M} - \frac{\hbar^2 \Delta_r}{2\mu} + \frac{1}{8} m_B \omega_B^2 r^2 + \frac{1}{2} m_B \omega_B^2 R^2 + \\ + g\delta(r) \frac{\partial}{\partial r} r - \frac{1}{2} m_B \omega_B^2 \mathbf{R} \cdot \mathbf{r}. \tag{7}$$

The separable part of this Hamiltonian consists of harmonic oscillator states in the center of mass, and parabolic cylinder functions in the relative motion which are coupled to each other by the term proportional to $\mathbf{R} \cdot \mathbf{r}$. One can then look at the system as a bound molecule placed in a harmonic potential with some internal structure. Resonances can be expected at the anticrossings between the levels with different number of excitation quanta stored in the center of mass motion. This leads to a series of confinement-induced resonances instead of just one. Most of these resonances will be very narrow as the coupling matrix element will be small. Away from the resonances the impact of coupling to the centre of mass only results in a small shift. The details of the trapping potentials will only slightly affect the couplings as they do not fundamentally change the shape of the wave functions. We thus see that the inclusion of the details of the trapping potential does not affect the properties of the system and does not impact the precision bounds that we predict. Accurate numerical modelling can even allow to utilize some of the very narrow resonances for magnetic field sensing. In recent years, efficient numerical methods have been developed [3, 8] which do not rely on the harmonicity of the traps or the initial conditions and should be appropriate for this task.

## II. LONG-RANGE INTERACTIONS

The second effect not included in the main part of this work is the possible impact on higher partial waves beyond the $s$-wave pseudopotential. This is particularly important for particles with long-range interactions such as the dipole-dipole one $U_{\rm dd}(r) = \frac{d^2}{r^3}\left(1 - 3(\hat{d} \cdot \hat{r})^2\right)$. When the interaction decays as $r^{-3}$, every partial wave allowed by symmetry contributes to the scattering [9]. Furthermore, the trapping potential also breaks the spherical symmetry and introduces couplings between partial waves. Multiple methods have been developed to handle this situation, including the short-range K matrix approach [10, 11]. Analytical treatments rely on separation of the length scales between the interaction and the trap width (the commonly used $s$-wave pseudopotential also relies on this assumption). In the short-range region only the interaction potential is relevant, the system is fully three-dimensional and the wave function is described using the short-range K matrix which contains all partial waves and includes the couplings between them coming from the anisotropic terms. In the long range, only the trapping potential is important and the wave function is again known. The matching between the two regions can be performed using the frame transformation technique [10, 11], which then allows for extracting the effective one-dimensional scattering amplitudes. The even part of the scattering contains contributions from all even partial waves, while the odd part contains all the odd ones.

The contribution of higher partial waves to the one-dimensional scattering has several possible effects. Firstly, diagonalization of the short-range K matrix including the coupling terms from the interaction results in a shift of the $s$-wave scattering length. This could be accounted for by using the actual value of the scattering length containing this shift in the bare $s$-wave pseudopotential. Furthermore, the higher partial waves result in emergence of additional poles in the one-dimensional K matrix which manifest themselves as additional resonances which are typically very narrow due to the repulsive centrifugal barrier which has to be tunnelled through. Finally, for the case of anisotropic interactions one encounters multiple resonances of mixed partial wave character. The theory of confinement-induced resonances in the presence of long-range interactions is well developed and allows for precise description of transmission properties as long as the free-space interaction is understood sufficiently well. The additional resonances do not diminish the performance of our sensor. For lanthanide atoms the dipolar interaction is rather weak and one can expect separation of length scales between the trap and the interaction. Even if this is not the case, numerical methods allow for using the realistic interatomic potentials along with the anharmonic trapping potentials [8, 12, 13].

This analysis combined with the one from the previous

section shows that even though the details of the trapping and interaction potentials result in multiple confinement-induced resonances coming from the coupling to the center of mass as well as higher partial waves, the fundamental properties of the system are captured by the simple model from the main part of the paper. The precision bounds we have derived for a single confinement-induced resonance remain valid for a realistic system, although one should expect that the actual position of the resonance can be somewhat shifted from the naive prediction.

## III. OPTIMAL MEASUREMENTS ON COLLIDING PARTICLES

In this section we show that the Fisher information $F$ calculated from the probability distribution corresponding to our proposed measurement scheme is equal to the quantum Fisher information $F_Q$ (QFI), which means that the performance of the sensor cannot be further improved by employing a different measurement scheme. The QCRLB, which provides the ultimate precision bound allowed by quantum mechanics, states that $F \leqslant F_Q$, where $F_Q$ is the maximum of the Fisher informations over all possible measurements. Thereforfe, the saturation of the QCRLB, i.e., $F = F_Q$, means that the considered measurement is optimal.

To show the optimality of our measurement scheme, we write the state of the single particle after the collision in the following form:

$$|\psi(B)\rangle = i\sin\delta_{1D} e^{i\delta_{1D}}|\psi_-\rangle + \cos\delta_{1D} e^{i\delta_{1D}}|\psi_+\rangle, \quad (8)$$

where $|\psi_\pm\rangle$ are the wavefunctions describing the transmitted/reflected particle, and $\delta_{1D}(B)$ is the one-dimensional phase shift given by Eq. (4) in the main text. An infinitesimal change from $B$ to $B + dB$ is accompanied by the change of the state from $|\psi(B)\rangle$ to $|\psi(B + dB)\rangle = e^{idB\hat{h}}|\psi(B)\rangle$, where $\hat{h}$ is the generator of the transformation [14], given by

$$\hat{h} = (\hat{1} + \hat{\sigma}_x)(\partial\delta_{1D}(B)/\partial B), \quad (9)$$

with the Pauli matrix $\hat{\sigma}_x$ expressed in the basis $|\psi_\pm\rangle$. The QFI is given by the variance of $\hat{h}$ on the state $|\psi(B)\rangle$, i.e.,

$$F_Q = 4(\langle\hat{h}^2\rangle - \langle\hat{h}\rangle^2). \quad (10)$$

Using the properties of the generator, we may write $F_Q = 4(\langle\psi|\psi'\rangle^2 + \langle\psi'|\psi'\rangle)$, where $|\psi'\rangle = \partial|\psi\rangle/\partial B$. A strightforward calculation gives then $F_Q = 4(\partial\delta_{1D}/\partial B)^2$, which is exactly $F$ in Eq. (6) in the main text after invoking that the transmission $T(B) = \cos^2\delta_{1D}(B)$.

This result can be understood from a different view. In Eq. (8), apart for the common phase factor $e^{i\delta_{1D}}$, the information about the phase shift $\delta_{1D}$ in the state $|\psi(B)\rangle$ is contained in the modulus of the probability amplitudes for finding the system in states $|\psi_\pm\rangle$. Accordingly, no information is contained in the phases of these amplitudes, and therefore, the measurement described by projection operators $|\psi_\pm\rangle\langle\psi_\pm|$, which leads to transmission/reflection probabilities, is optimal [15].

Now we show that $F$ cannot be increased by preparing a different initial state of the system, neither by introducing a phase reference (a superposition with a state that is independent of the magnetic field) nor by preparing a simple superposition of a particle injected into the opposite sides of the tubes. In the state $|\psi(B)\rangle$, see Eq. (8), the common phase can be factored out $|\psi(B)\rangle = e^{i\delta_{1D}}|\psi_0(B)\rangle$ with $|\psi_0(B)\rangle = i\sin\delta_{1D}(B)|\psi_-\rangle + \cos\delta_{1D}(B)|\psi_+\rangle$. The common phase cannot be detected, because it cancels when calculating the probabilities of any observable. The information that is encoded in that phase is lost. However, consider now a superposition of state $|\psi(B)\rangle$ and $|\psi_1\rangle$, as for example in $e^{i\delta_{1D}}|\psi_0(B)\rangle + |\psi_1\rangle$. Here the state $|\psi_1\rangle$ serves as a phase reference, so the superposition is now sensitive to the phase $e^{i\delta_{1D}}$. The question is, whether such a superposition yields a better precision. Now, we show that it cannot be the case. To this end, we calculate the QFI for a general state $|\phi\rangle = c_0|\psi_0\rangle + c_1|\psi_1\rangle$ with arbitrary amplitudes $c_0$ and $c_1$, and states $|\psi_0\rangle$ and $|\psi_1\rangle$. We assume that only $|\psi_0\rangle$ is affected by the generator $\hat{h}$ whereas the state $|\psi_1\rangle$ is not. The QFI is then given by $F_Q[|\phi\rangle] = \gamma F_Q[|\psi_0\rangle] + 4\gamma(1-\gamma)\langle\hat{h}\rangle_0^2$, where $\gamma = |c_0|^2$ and $\langle\cdot\rangle_0$ stands for the average over the state $|\psi_0\rangle$. Using the fact that eigenvalues of $\hat{h}$ are 0 and $2(\partial\delta_{1D}(B)/\partial B)$, one has $F_Q = 4\gamma(\langle\hat{h}^2\rangle_0 - \langle\hat{h}\rangle_0^2) + 4\gamma(1-\gamma)\langle\hat{h}\rangle_0^2 \leqslant 4(\partial\delta_{1D}(B)/\partial B)^2$ regardless of the state. Therefore, superposition with a phase reference cannot help. Moreover, this inequality is already saturated with our setup, see Eq. (6) in the main text. As a consequence, to enhance the sensitivity it is necessary to use initial states that are entangled.


[1] F. Werner, L. Tarruell, and Y. Castin, The European Physical Journal B **68**, 401 (2009).

[2] K. Jachymski, F. Meinert, H. Veksler, P. S. Julienne, and S. Fishman, Phys. Rev. A **95**, 052703 (2017).

[3] S. Sala, P.-I. Schneider, and A. Saenz, Phys. Rev. Lett. **109**, 073201 (2012).

[4] S. Sala and A. Saenz, Phys. Rev. A **94**, 022713 (2016).

[5] M. Olshanii, Phys. Rev. Lett. **81**, 938 (1998).

[6] P. Massignan and Y. Castin, Phys. Rev. A **74**, 013616 (2006).

[7] M. Wouters and G. Orso, Phys. Rev. A **73**, 012707 (2006).

[8] V. S. Melezhik, J. I. Kim, and P. Schmelcher, Phys. Rev. A **76**, 053611 (2007).

[9] H. Sadeghpour, J. Bohn, M. Cavagnero, B. Esry, I. Fabrikant, J. Macek, and A. Rau, Journal of Physics B: Atomic, Molecular and Optical Physics **33** (2000).

[10] P. Giannakeas, V. S. Melezhik, and P. Schmelcher, Phys. Rev. Lett. **111**, 183201 (2013).

[11] B. Heß, P. Giannakeas, and P. Schmelcher, Phys. Rev. A **92**, 022706 (2015).

[12] V. S. Melezhik and A. Negretti, Phys. Rev. A **94**, 022704 (2016).

[13] B. Schulz, S. Sala, and A. Saenz, New Journal of Physics **17**, 065002 (2015).

[14] S. L. Braunstein and C. M. Caves, Phys. Rev. Lett. **72**, 3439 (1994).

[15] T. Wasak, A. Smerzi, L. Pezzé, and J. Chwedeńczuk, Quantum information processing **15**, 2231 (2016).
